# Supplementary material for: Observation of a dynamic magneto-chiral instability in photoexcited tellurium
Source: arXiv:2502.05170 source file (2025-02-07)
Supplement: Supplementary file 1 [file Te_THz_SI.pdf]

# Supplementary Information
# Observation of a dynamic magneto-chiral instability in photoexcited tellurium

Yijing Huang,[1,2,*] Nick Abboud,[3,*] Yinchuan Lv,[1,2] Penghao Zhu,[1,4,5] Azel Murzabekova,[1,2] Changjun Lee,[6,2] Emma A. Pappas,[1,2] Dominic Petruzzi,[1,2] Jason Y. Yan,[1,2] Dipanjan Chauduri,[1,2] Peter Abbamonte,[1,2] Daniel P. Shoemaker,[6,2] Rafael M. Fernandes,[1,4] Jorge Noronha,[3] and Fahad Mahmood[1,2]

[1]*Department of Physics, The Grainger College of Engineering, University of Illinois Urbana-Champaign, Urbana, Illinois 61801, USA*
[2]*Materials Research Laboratory, The Grainger College of Engineering, University of Illinois Urbana-Champaign, Urbana, Illinois 61801, USA*
[3]*Illinois Center for Advanced Studies of the Universe and Department of Physics, The Grainger College of Engineering, University of Illinois Urbana-Champaign, Urbana, Illinois 61801, USA*
[4]*Anthony J. Leggett Institute for Condensed Matter Theory, The Grainger College of Engineering, University of Illinois Urbana-Champaign, Urbana, Illinois 61801, USA*
[5]*Department of Physics, The Ohio State University, Columbus, OH 43210, USA*
[6]*Department of Materials Science and Engineering, The Grainger College of Engineering, University of Illinois Urbana-Champaign, Urbana, Illinois 61801, USA*

## CONTENTS

A. Robustness of the Linear Prediction Algorithm 2

B. Optical Pump-Probe Reflectivity 6

C. Band Structure of Tellurium and Impurity Levels 7

D. Longer Delay THz emission Scan 8

E. The Model of a Magneto-Chiral Instability 10

References 15

---

* These authors contributed equally to this work.

## A. ROBUSTNESS OF THE LINEAR PREDICTION ALGORITHM

Linear prediction decomposes the data presumably of the form $\sum_i A_i e^{\beta_i t}\cos(\omega_i t+\phi_i)$ into harmonic oscillators with exponential factors [1]. It gives a statistically sound estimate of the number of oscillators ($K$) in the signal [2, 3]. As a fit in the time-domain, it extracts $\beta_i > 0$ modes, which is not possible using the more conventional fit to the Fourier-domain data assuming a sum of decaying ($\beta < 0$) harmonic oscillators (Lorentzians). A brief description of the procedure of the algorithm is provided here, following the recipe described in Ref [1]. If the time-domain data is of length $N$, then one can pick any time point of index $n$, and the signal at this particular time can be predicted using the signals from previous $M$ time points (hence the name linear prediction).

$$x_n = a_1 x_{n-1} + a_2 x_{n-2} + a_3 x_{n-3} + ... + a_M x_{n-M}, \tag{1}$$

and $n$ can take any value from $M+1$ to $N$, in total $N-M$ integers. The series of $a_n$ can be obtained through singular value decomposition of the $(N-M)\times M$ matrix formed entirely by data values at different time points [1]. For noiseless data consisting $K$ harmonic oscillators, the model parameters $(A_i, \beta_i, \omega_i, phi_i)$ can be obtained by solving roots of a $2K$-order polynomial with the polynomial coefficients $a_n$. The procedure accurately extracts oscillator parameters as long as $M > 2K$. Unlike least-squares fitting, linear prediction requires no initial input and provides a unique, deterministic solution. The algorithm is mathematically robust for noise-free data, ensuring it neither misses harmonic components nor overfits.

In practice, the data is corrupted by noise, and linear prediction may attempt to capture components near or below the noise level, resulting in low confidence when fitting near-noise-level components, just as with any fitting routine. Based on the distribution of singular values, one can set the rank $r$ ($< M$), which is the number of significant singular values in the singular value decomposition. The remaining insignificant singular values are considered contributions from noise [2, 3]. For systems without persistent energy input, sinusoidal harmonics with $\beta_i > 0$ are unphysical, thus any components with $\beta_i > 0$ should be discarded [1]. In fact, for these systems, $\beta_i > 0$ components are purely artifacts of overfitting, they should be below the noise level and would correspond to insignificant singular values with indices larger than the rank $r$. The algorithm has been proven robust for nuclear magnetic resonance spectroscopy (NMR) [4] and ultrafast pump-probe measurements [5–7] for data of decent signal-noise-ratio that is truly a combination of *decaying* oscillators. For systems with external energy input allowing $\beta_i > 0$ components, the above recipe remains effective and is applied to our experimental data. Take the data with $\boldsymbol{B}_0 \parallel \mathbf{c}$ sample orientation for example. The rank needs to be moderately large ($\sim 20$) to ensure that $r > 2K$ ($K$=5 according to the results) and avoid frequency bias [8]. With over 130 data points in the selected time window, the choice of $M = 0.5 \times N$ ensures $M$ is much larger than the chosen rank $r$, which guarantees that $2K < r < M$. If the fit yields components that are an order of magnitude smaller than the more significant components, or are comparable to either the noise level or the fit residual, it would indicate that $r$ could have been chosen to be a smaller number and that these components can be considered noise and discarded.

We first constrain that $\beta_i < 0$ for all $i$, as shown in Fig. S1(a-d). In Fig. S1(a), we show the time-domain data taken in the $\boldsymbol{B}_0 \parallel \mathbf{c}$ orientation. The blue curve is the raw data, the green curve is the linear prediction constraining $\beta_i < 0$ for all $i$. The residual (red curve) is of significant amplitude and implies the presence of components that increase in amplitude over time. The residual indicates that the linear prediction algorithm enforcing $\beta_i < 0$ for all $i$ does not capture the data. Fig. S1(b) is the Fourier transform of the time traces in Fig. S1(a), which shows that the large residual (red curve) has a frequency of approximately 0.37 THz. Fig. S1(c) shows the time-domain traces for the $\boldsymbol{B}_0 \perp \mathbf{c}$ sample orientation. The color code is the same as in Fig. S1(a). The corresponding Fourier transform in Fig. S1(d) reveals that the red residual comprises of multiple frequencies that do not satisfy $\beta_i < 0$.

In Fig. S1(e-h), we show the same data as in Fig. S1(a-d), however, here we do not constrain that $\beta_i < 0$ for all $i$ in the linear prediction algorithm. In Fig. S1(e), the green trace is the linear prediction result after selecting the significant components. The amplitudes of the non-selected components are at least one order of magnitude smaller than that of the selected components. Here a total of five sinusoidal harmonic components are selected. The red curve is the residual, which is on the noise floor. In Fig. S1(f), we show the Fourier transform of the curves in Fig. S1(e) with the same color code. The data with $\boldsymbol{B}_0 \perp \mathbf{c}$ orientation, which is of much higher signal-noise ratio than $\boldsymbol{B}_0 \parallel \mathbf{c}$ data, is presented in Fig. S1(g-h) with the same color code as in Fig. S1(e-f). We also performed least squares fitting using the oscillator parameters obtained above as the initial input and found good agreement with the data with minimal changes to the final fit parameters. We conclude that the linear prediction algorithm provides a reasonable description of the data.

We next examine the individual frequency components extracted from the linear prediction algorithm for both sample orientations, in addition to those presented in Main Text Fig. 3. The robustness of the linear prediction algorithm is evident from the systematic temperature and field dependence, as well as the consistent initial phases of the components observed across varying external magnetic fields and temperatures.

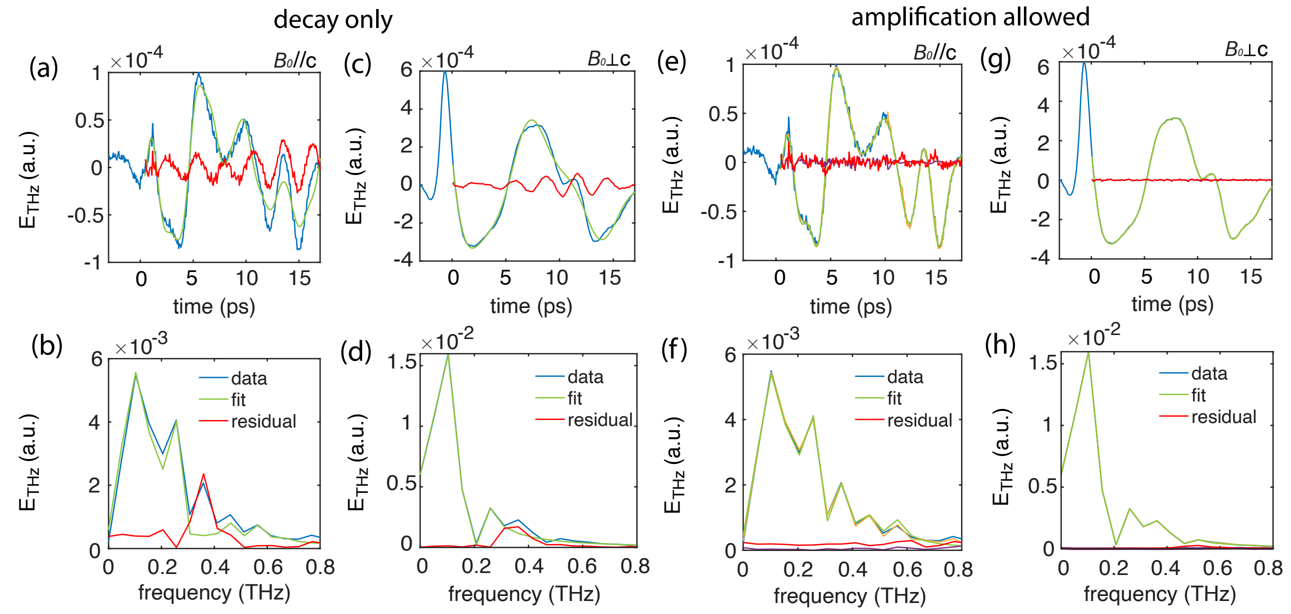


Fig. S1. **Linear prediction algorithm applied to $s$-polarized THz emission $S_{\mathbf{odd}}$.** (a) Time-domain data with the $\boldsymbol{B}_0 \parallel \mathbf{c}$ sample orientation (blue). The green curve shows the data's linear prediction (also called "fit", doubled quoted since there is no optimization in the algorithm) when only $\beta_i$ <0 components are allowed in the solution. The red curve shows the residual. (b) The Fourier transform of the time traces in (a). (c-d) Same as (a-b) but for data taken in the $\boldsymbol{B}_0 \perp \mathbf{c}$ configuration. (e) shows the same data as in (a) with the sample orientation $\boldsymbol{B}_0 \parallel \mathbf{c}$, but using a linear prediction algorithm that does not constrain all $\beta_i$ <0. The "fit" selects the significant components (at least an order of magnitude larger than the rest of the non-selected components) of the linear prediction results and is shown in the green curve. The red curve is the "fit" residual. (f) Fourier transform of (e). The red contains more spectral components than the purple trace, which is expected. (g-h) The same as in (e-f) but for the sample orientation $\boldsymbol{B}_0 \perp \mathbf{c}$.

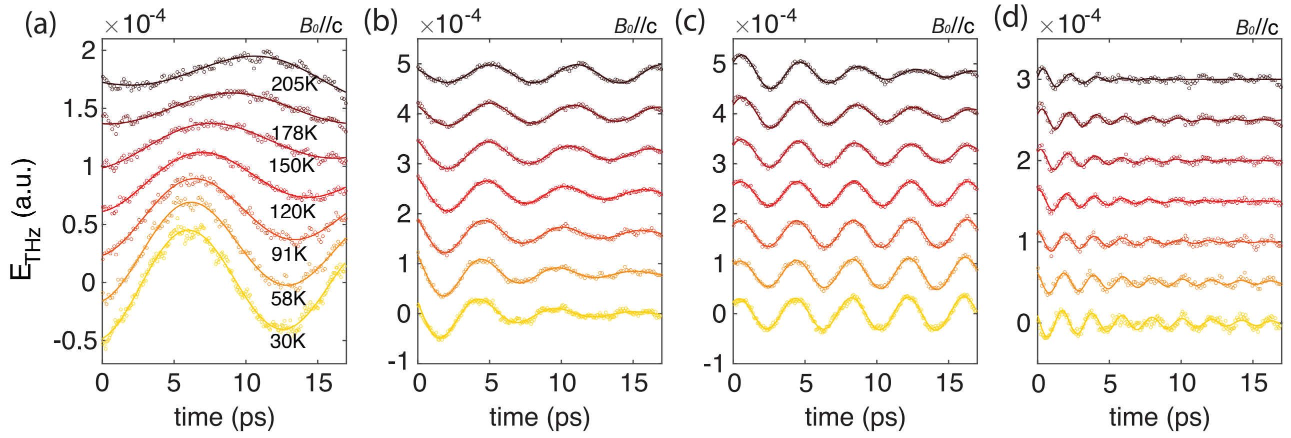


Fig. S2. **Temperature dependence of frequency components in $s$-polarized THz emission $S_{\mathbf{odd}}$, measured in the $\boldsymbol{B}_0 \parallel \mathbf{c}$ sample orientation (at 6 T).** Each plot is made for one frequency component. The colored circles represent the raw data subtracted by all other components, the solid lines represent the one selected component. (a) The plot for the < 0.1 THz mode. (b) The plot for the 0.16 THz mode. (c) The plot for the 0.26 THz mode. (d) The plot for the 0.5 THz mode.

In Fig. S2, we show the temperature dependence of different frequency components of the $\boldsymbol{E}_s$ emissions with the $\boldsymbol{B}_0 \parallel \mathbf{c}$ sample orientation at 6 T. For each plot, we pick the target frequency component(s). The solid lines represent the selected component(s), whereas the colored circles represent the raw data subtracted by all other components. Fig. S2(a) shows the < 0.1 THz mode, Fig. S2(b) the 0.16 THz mode, Fig. S2(c) the 0.26 THz mode, and Fig. S2(d) the 0.5 THz mode. The signal to noise ratio is quite good - all the extracted components are well above the noise level. The initial phase of each trajectory is consistent within the temperature range of

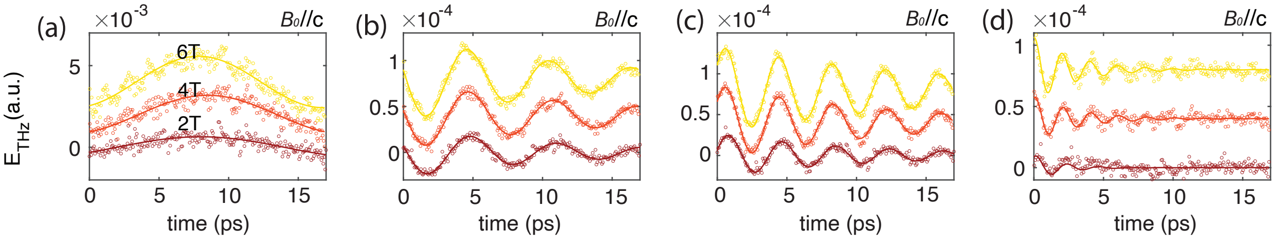


Fig. S3. **The field dependence of frequency components in $s$-polarized THz emission $S_{\mathrm{odd}}$, measured in the $\boldsymbol{B}_0 \parallel$ c sample orientation (at 17 K).** Each plot is made for one frequency component. The colored circles represent the raw data subtracted by all other components, the solid lines represent the one selected component. (a) The plot for the $< 0.1$ THz mode. (b) The plot for the 0.16 THz mode. (c) The plot for the 0.26 THz mode. (d) The plot for the 0.5 THz mode.

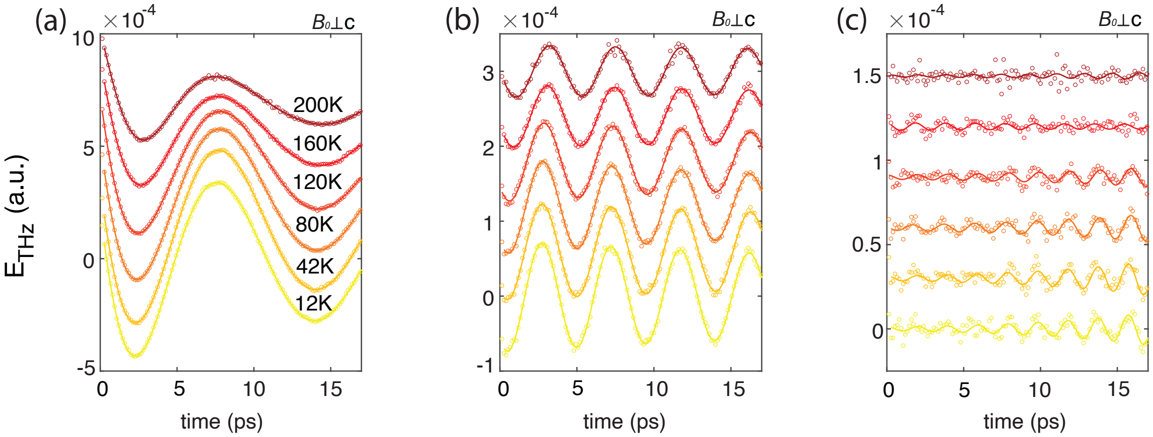


Fig. S4. **Temperature dependence of frequency components in the $s$-polarized THz emission $S_{\mathrm{odd}}$, measured with the $\boldsymbol{B}_0 \perp$ c sample orientation (at 6 T).** The solid lines represent the selected frequency components. The colored circles represent the raw data subtracted by all other modes. (a) The plot for the $< 0.1$ THz components. (b) The plot for the 0.22 THz mode. (c) The plot for the 0.5 THz mode.

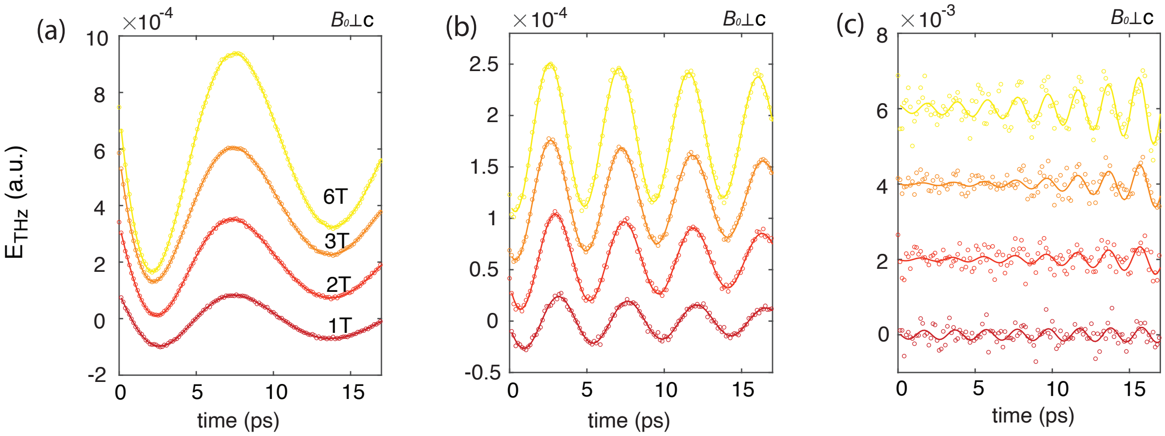


Fig. S5. **The field dependence of frequency components in $s$-polarized THz emission $S_{\mathrm{odd}}$, measured with the $\boldsymbol{B}_0 \perp$ c sample orientation (at 12 K).** The solid lines represent the selected frequency components. The colored circles represent the raw data subtracted by all other modes. (a) The plot for the $< 0.1$ THz components. (b) The plot for the 0.22 THz mode. (c) The plot for the 0.5 THz mode.

the experiment.

Fig. S3 shows the $\boldsymbol{B}_0$ field dependence (at 17 K) of the same frequency components as in Fig. S2. Except for the $< 0.1$ THz mode, the other frequency components maintain consistent initial frequencies and phases with those in the temperature dependence scan in Fig. S2. The differing frequency and phase of the $< 0.1$ THz component between 17 K and 30 K (at 6 T) is attributed to the potential systematic experimental difference of different thermal cycles and the highly nonlinear nature of THz emission, consistent with the increase in $\beta$ of the 0.37 THz mode from 17 K and 30 K in Fig.3(h) of the Main Text, which is an outlier to the general temperature dependence of $\beta$ for the 0.37 THz mode in the $\boldsymbol{B}_0 \parallel \mathbf{c}$ orientation.

In Fig. S4 we show the temperature dependence of frequency components of $\boldsymbol{E}_s$ emissions with $\boldsymbol{B}_0 \perp \mathbf{c}$ sample orientation (at 6 T). Fig. S4(a-c) show the $< 0.1$ THz components, the 0.22 THz mode and the 0.5 THz mode, respectively. The $< 0.1$ THz components contain sinusoidal harmonics at two slightly different frequencies around 0.07 THz with a frequency spacing of $\approx 10$ GHz [see Main Text Fig.2(b)], which can be attributed to chirp, a frequency change over time, discernible in the time-domain trace of Fig. S4(a)]. The 0.5 THz component shows some amplification over time but is close to the noise level and has an amplitude an order of magnitude smaller than the other sinusoidal components. Therefore, we do not assign it a high confidence of fit. Fig. S5 shows the field dependence (at 12 K) of the same frequency components as in Fig. S4.

Here we make important comments on the frequency resolution of the experimental data as processed by the linear prediction algorithm. With a limited frequency resolution, a mode may appear to increase its amplitude over time with an amplification constant $\beta$ due to a pair of modes with frequencies $\approx f_0$ slightly separated by $\Delta f \approx \frac{\beta}{2\pi}(\ll f_0)$, given that they start oscillating with similar amplitudes but nearly out of phase. We estimate the order of magnitude of $\beta \approx 0.1$ ps$^{-1}$ at lower temperatures (<30 K) and the highest experimentally accessible $|\boldsymbol{B}_0|$ (6 T) based on Main Text Fig.3(h-j). This corresponds to a $\Delta f \approx 16$ GHz if the amplification is due to beating. We note that though the frequency resolution can be influenced by noise, the linear prediction algorithm is not constrained by the Nyquist–Shannon sampling theorem [1]. The latter states that the frequency resolution cannot exceed $\frac{1}{2T}$ where $T$ is the scan time window, and thus suggests that Fourier domain analysis of data over a 17 ps time window cannot resolve frequency-proximate modes with $\Delta f$ <30 GHz. However, the linear prediction algorithm resolves $\Delta f$ <10 GHz modes for data of a 1 ps time window [Main Text Fig.3(d) right panel, Fig. S5(a) and Fig. S4(a)] due to its sensitivity to amplitudes and phases of modes in addition to their frequencies. In NMR spectroscopy, this point is well-established: comparison between the Fourier spectra of raw data and the Fourier spectra of the linear prediction-extracted free induction decay shows that the Fourier peak width is significantly reduced using linear prediction algorithm [4]. Therefore, our fitting routine does not confuse a $\Delta f \approx 16$ GHz beating with an amplification rate $\beta \approx 0.1$ THz. We also note that none of the extracted resonance frequencies match the multiple or sum of other resonance frequencies, ruling out a parametric amplification mechanism, where modes can be amplified if they couple nonlinearly to other driven modes [9].

## B. OPTICAL PUMP-PROBE REFLECTIVITY

We performed time-resolved 1030 nm pump and 515 nm probe reflectivity measurements of tellurium, with the $\boldsymbol{B}_0 \parallel \mathbf{c}$ sample orientation at 10 K. The results are shown in Fig. S6. The reflectivity probe does not have a special detection scheme such as optical birefringence or dichroism using a polarizing beam splitter [10], and should correspond to the "isotropic" Raman channel reported in Refs [11, 12], which show a Raman-active phonon at just below 4 THz. Such a phonon is on the verge of our experimental resolution and is not observed here.

The optical reflectivity in Fig. S6(a) shows no significant dependence on $|\boldsymbol{B}_0|$. And Fig. S6(b) suggest no significant change upon flipping the $\boldsymbol{B}_0$ polarity, under different fluences. Unlike the THz emission data, the pump-probe reflectivity data presented here is not $\boldsymbol{B}_0$-antisymmetrized. These optical reflectivity measurements suggest that the resonances observed in Main Text Fig. 2(a) and (d) are not Raman-active.

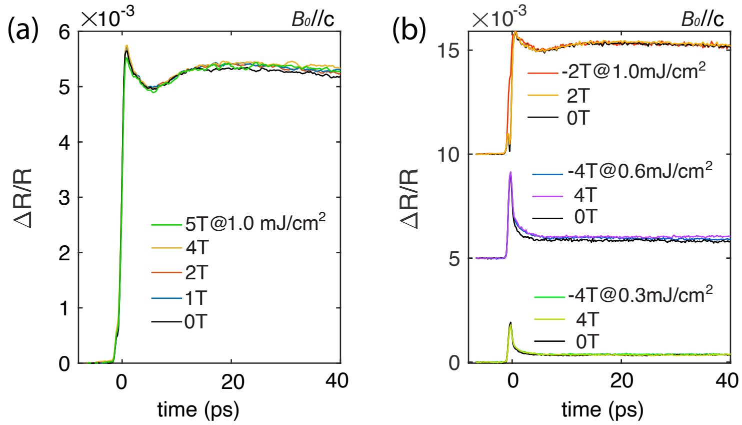


Fig. S6. **Optical pump-probe reflectivity of tellurium under $\boldsymbol{B}_0$ field at 10 K.** (a) The optical (1030 nm) pump- (515 nm) probe reflectivity of tellurium under different $\boldsymbol{B}_0$ fields. (b) The optical (1030 nm) pump- (515 nm) probe reflectivity of tellurium under the different $\boldsymbol{B}_0$ polarity and under different fluences.

## C. BAND STRUCTURE OF TELLURIUM AND IMPURITY LEVELS

Part of the tellurium electron band structure [13] as well as a schematic of its Brillouin zone is provided in Fig. S7 (a).The lowest-energy direct-bandgap transition occurs at the $H$ point (and its time reversal point $H$'). Four acceptor states near the valence band $H_4$ and one near the valence band $H_5$, were previously identified in Refs [14–17]. According to Ref [15], the energy separation between the first (second) acceptor state and the top of the $H_4$ valence band [top of the camel back in Fig. S7(b)] is 1.21 meV (0.86 meV) which is approximately 0.29 THz (0.21 THz). In Ref [17], the calculated corresponding value is 1.29 meV (0.9 meV) which is approximately 0.31 THz (0.22 THz). Ref [14] identifies an acceptor level 0.2 meV, which is about 0.05 THz above the valence band maximum at $H_4$, whereas Ref [16] identifies one at 0.37 meV, which is about 0.09 THz below the valence band maximum at $H_4$. Additionally, Ref [15] assigns another acceptor state 1.26 meV (0.30 THz) above the top of the $H_5$ valence band. These energy scales are consistent with our observed THz emissions and are summarized in Fig. S7(b). The exact resonance frequencies depend on the impurity type. The lack of $\boldsymbol{B}_0$ dependence of resonance frequencies is attributed to the large effective mass of the acceptor states, and the differences of mode frequencies between the $\boldsymbol{B}_0 \parallel \mathbf{c}$ and $\boldsymbol{B}_0 \perp \mathbf{c}$ sample orientations [see Main Text Fig.2 (a) and (d)] is attributed to the anisotropy of the effective mass of impurity-level electrons. Even high-purity tellurium with a dopant density as low as $10^{14}$ cm$^{-3}$ can produce signatures of acceptor states in magnetotransmission experiments [14]. We note that X-ray fluorescence spectroscopy with a sensitivity of 0.1 ppm (corresponding to an estimated impurity density of $10^{16}$ cm$^{-3}$) cannot assign the impurity element for the sample used in our THz emission experiments.

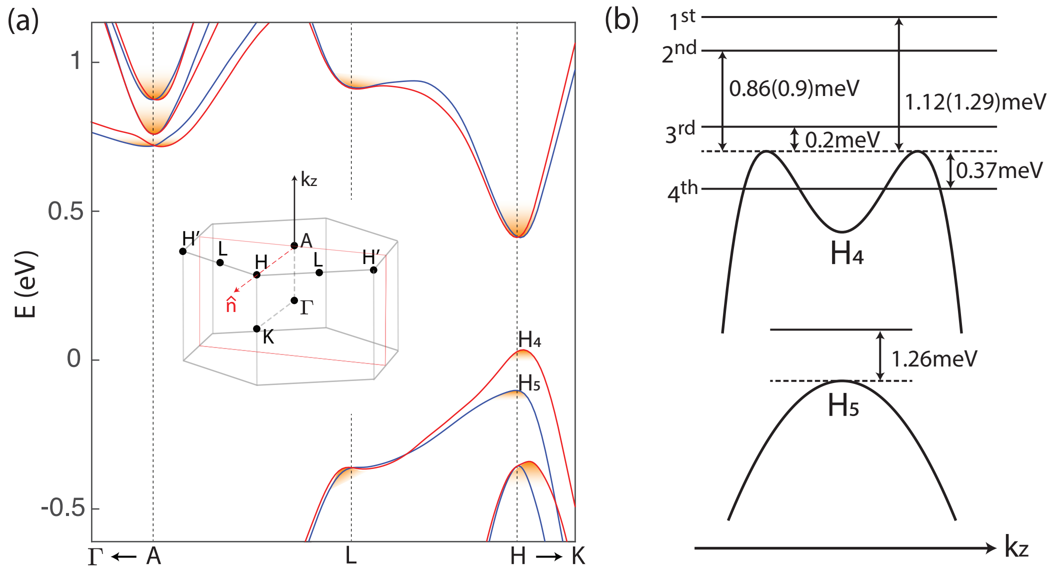


Fig. S7. **Band structure and impurity diagram of tellurium.** (a) Part of the tellurium electron band structure. The band structure is adapted from Ref [13] with authorization via license CC BY 4.0 [18]. The inset shows the Brillouin zone, with high-symmetry points marked. $\hat{n}$ denotes the sample normal whereas the red contour denotes the sample surface. (b) The energy diagram of impurity levels.

The $\boldsymbol{B}_0$ field breaks time-reversal and may split the impurity level by lifting the degeneracy of the $H$ and $H'$ valleys. Previous GHz-(0.01 meV)-frequency-resolution photoconductivity experiment [19] reported the absence of magnetic-field-induced energy level splitting ($\Delta f < 1$ GHz, the experimental resolution) in $\boldsymbol{B}_0 \perp \mathbf{c}$ orientation (at 1.4 K) up to 6 T. This report rules out an artifact amplification due to a pair of modes launched out-of-phase with frequencies $\approx f_0$ slightly separated by $\Delta f \approx \frac{\beta}{2\pi}(\ll f_0)$, since $\Delta f \lesssim 1$ GHz which is more than an order of magnitude smaller than the $\beta$ (corresponding to 16 GHz) measured under comparable temperatures and fields, see Main Text Fig.3(h-j). Even if acceptor levels of different chemical elements are accidentally frequency-proximate, resonances due to acceptor states obtained from the same form of low-energy Hamiltonian are not expected to be launched out of phase.

## D. LONGER DELAY THZ EMISSION SCAN

The data presented in the Main Text uses a (110)-cut CdTe EO sampling crystal which produces an echo at around 20 ps due to the reflection inside CdTe. Here, by replacing the (110)-cut CdTe with a stack of a (110)-cut CdTe and a (100)-cut CdTe of the same thickness, we greatly mitigate the first reflection from the (110)-cut CdTe surface so that the echo-free scan range can be doubled. See Fig. S8(a) and (b) for $\boldsymbol{E}_s$ and $\boldsymbol{E}_p$ under the $\tilde{\boldsymbol{E}}_s$ pump. In Fig. S8(a) and (b), for the non-zero magnetic fields, the colored curves show the $\boldsymbol{B}_0$-antisymmetrized data $S_{\mathrm{odd}}$, whereas the black curves show the $\boldsymbol{B}_0$-symmetrized data. The echo reduction is not perfect, as can be seen from Fig. S8(a) black curves near 20 ps. Fig. S8(c), which is the Fourier transform of Fig. S8(a) for the 35 ps time window starting at 5 ps, shows the five frequency peaks, which are consistent with the extraction of linear prediction algorithm from a shorter time window in the Main Text (Fig.2). Fig. S8(d), which is the Fourier transform of Fig. S8(b), shows that $\boldsymbol{E}_p$ is comparable to $\boldsymbol{E}_s$ in amplitude within the 35 ps time window after 5 ps.

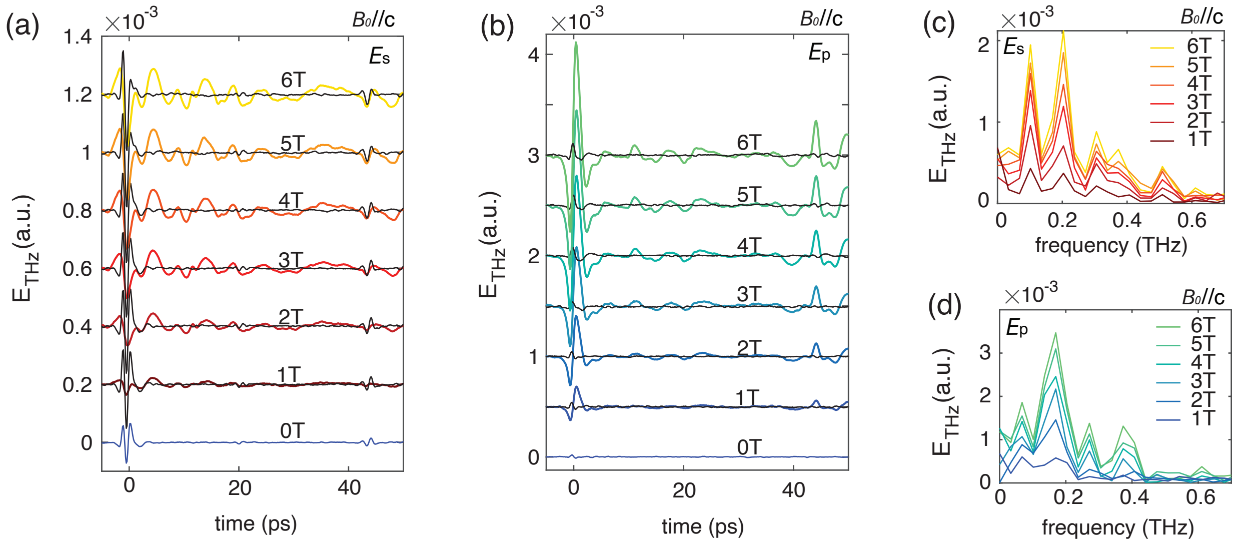


Fig. S8. **The longer scans of $\boldsymbol{B}_0$ dependent THz emissions under the $\tilde{\boldsymbol{E}}_s$ pump.** (a) The $\boldsymbol{E}_s$ emissions under different magnetic fields (0 T to 6 T). The black lines of the $\boldsymbol{B}_0 \neq \boldsymbol{0}$ scans show the $\boldsymbol{B}_0$-symmetrized data, and there is a reduced pulse reflection at the interface of the (110)-cut CdTe and the (100)-cut CdTe at around 20 ps. The major echo reflection is beyond 40 ps. (b) The $\boldsymbol{E}_p$ emissions under different magnetic fields (0 T to 6 T). (c) Fourier transform of (a) between 5 ps and 40 ps. (d) Fourier transform of (b) between 5 ps and 40 ps.

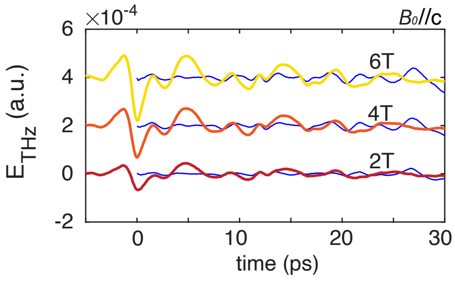


Fig. S9. **Linear prediction algorithm performed on longer scans of $\boldsymbol{E}_s$ THz emissions from the $\tilde{\boldsymbol{E}}_s$ pump.** Linear prediction algorithm performed on 30 ps scans of $\boldsymbol{E}_s$ THz emissions (colored curves) yields large residuals (blue curves).

In Fig. S9, the linear prediction algorithm is performed over a 30 ps time window for the data taken under the $\boldsymbol{B}_0 \parallel \mathbf{c}$ configuration. Though the Fourier transforms of the $\boldsymbol{E}_s$ over a 35 ps (5 ps - 40 ps) time window clearly shows five frequency peaks in Fig. S8(c), linear prediction of the 30 ps $\boldsymbol{E}_s$ THz emission in Fig. S9 yields quite

large residuals (blue curves) despite the reasonable signal-to-noise ratio of the data, in contrast to the negligible residual in Main Text Fig. 2 and SI Fig. S1(e),(g). Though a shorter time window (for example, 0-15 ps) does reveal the unstable mode, the linear prediction algorithm does not decompose the long-scan 0-30 ps data in Fig. S9 into sinusoids. This suggests that, between 20-30 ps, the data can no longer be accurately described using a sum of sinusoids with fixed exponential factors $\beta_i$. From this, we infer that $\sigma_{\mathrm{M}}$, as defined in Main Text Eq.(3), decays within 20-30 ps. We note that 30 ps is the time scale that $> 99\%$ photoexcited carriers in tellurium recombine, according to Ref [13]. The absence of a beating "revival" also does not support beating as an explanation for the amplified mode in Main Text Fig. 3.

## E. THE MODEL OF A MAGNETO-CHIRAL INSTABILITY

In this section, we describe the construction of the model employed in the Main Text, starting from Maxwell's equations and a linear response expression for the current density. We work with the electromagnetic potential $A^\mu$ in a temporal gauge, i.e. $A^0 = 0$. The electric and magnetic fields are $\boldsymbol{E} = -\partial_t \boldsymbol{A}$ and $\boldsymbol{B} = \boldsymbol{\nabla} \times \boldsymbol{A}$, respectively, and Maxwell's equations read

$$-\nabla^2 \boldsymbol{A} + \boldsymbol{\nabla}(\boldsymbol{\nabla} \cdot \boldsymbol{A}) = \mu_0(\boldsymbol{j} - \epsilon \partial_t^2 \boldsymbol{A}), \tag{2}$$

$$-\boldsymbol{\nabla} \cdot \partial_t \boldsymbol{A} = \rho/\epsilon_0, \tag{3}$$

where $\epsilon = \epsilon_r \epsilon_0$ is the in-medium permittivity. Once Eq. (2) is solved for $\boldsymbol{A}$, Eq. (3) determines the charge density $\rho(\boldsymbol{r}, t)$, which is therefore not an independent dynamical degree of freedom from $\boldsymbol{A}$.

Inserting the plane-wave ansatz $\boldsymbol{A}(\boldsymbol{r}, t) = \boldsymbol{A}(\omega, \boldsymbol{k}) e^{i(\boldsymbol{k}\cdot\boldsymbol{r} - \omega t)}$ and putting

$$\boldsymbol{j}(\omega, \boldsymbol{k}) = \sigma_{\mathrm{E}}(\omega) \boldsymbol{E}(\omega, \boldsymbol{k}) + \sigma_{\mathrm{M}}(\omega) \boldsymbol{B}(\omega, \boldsymbol{k}), \tag{4}$$

Eq. (2) becomes

$$\mathbb{M}\boldsymbol{A} = 0, \qquad \mathbb{M} = \epsilon \left(\omega^2 - v^2 k^2\right) \mathbb{1} + \epsilon v^2 \boldsymbol{k}\boldsymbol{k}^\intercal + i\omega\sigma_{\mathrm{E}}(\omega) + i\sigma_{\mathrm{M}}(\omega)\mathbb{K}, \tag{5}$$

where $v = 1/\sqrt{\mu_0 \epsilon}$ is the in-medium speed of light, $k = |\boldsymbol{k}|$, and $\mathbb{K}\boldsymbol{A} \equiv \boldsymbol{k} \times \boldsymbol{A}$. The dispersion relations $\omega(k)$ are then obtained as the solutions of $\det \mathbb{M} = 0$, and they depend only on $k = |\boldsymbol{k}|$. We note that one pure gauge degree of freedom remains in the temporal gauge, which manifests itself here as a spurious solution $\boldsymbol{A}(\omega, \boldsymbol{k})$ for which $\boldsymbol{E}(\omega, \boldsymbol{k}) = 0$ and $\boldsymbol{B}(\omega, \boldsymbol{k}) = 0$, i.e. for which $\omega(k) = 0$ and $\boldsymbol{A} \propto \boldsymbol{k}$. Among the *non*-spurious solutions, those with $\boldsymbol{A} \propto \boldsymbol{k}$ correspond to transverse, purely electric modes of the form $\boldsymbol{E}(\boldsymbol{r}, t) \propto \frac{\boldsymbol{k}}{k} e^{i(\boldsymbol{k}\cdot\boldsymbol{r} - \omega t)}$ with $\boldsymbol{B} = 0$, where $\omega$ is a ($k$-independent) solution of $\epsilon_r \epsilon_0 \omega = -i\sigma_{\mathrm{E}}(\omega)$. These modes are stable ($\mathrm{Im}[\omega] < 0$) and will not be discussed further.

One finds that the remaining dispersion relations are the solutions of

$$\epsilon(\omega^2 - v^2 k^2) + i\omega\sigma_{\mathrm{E}}(\omega) + \lambda\sigma_{\mathrm{M}}(\omega) k = 0. \tag{6}$$

These solutions can be written as $\omega_{\lambda s}(k)$, with $s$ labeling the different branches, and $\lambda = \pm 1$. The corresponding modes are circularly polarized waves with helicity $\lambda$, namely

$$\boldsymbol{E}_{\lambda s \boldsymbol{k}}(\boldsymbol{r}, t) = i\omega_{\lambda s}(k) \left[\boldsymbol{e}_1(\boldsymbol{k}) + i\lambda \boldsymbol{e}_2(\boldsymbol{k})\right] e^{i(\boldsymbol{k}\cdot\boldsymbol{r} - \omega_{\lambda s}(k) t)}, \tag{7a}$$

$$\boldsymbol{B}_{\lambda s \boldsymbol{k}}(\boldsymbol{r}, t) = -i\lambda \frac{k}{\omega_{\lambda s}(k)} \boldsymbol{E}_{\lambda s \boldsymbol{k}}(\boldsymbol{r}, t), \tag{7b}$$

where $\boldsymbol{e}_1(\boldsymbol{k})$, $\boldsymbol{e}_2(\boldsymbol{k})$, and $\boldsymbol{k}/k$ form a right-handed orthonormal basis.

Below we present a progression of current-density linear response models that lead up to the model discussed in the Main Text. Note that single-crystal tellurium does not have chiral domains [20–22], therefore $\sigma_{\mathrm{M}}$ as a chiral order parameter is uniform within the NIR laser-illuminated region.

**Ohmic conduction.** First, we consider the case of Ohmic conduction, $\sigma_{\mathrm{E}}(\omega) = \sigma_{E0}$ and $\sigma_{\mathrm{M}}(\omega) = 0$, where $\sigma_{E0}$ is constant. The dispersion relations from Eq. (6) are

$$\omega_s(k) = -\frac{i\sigma_{E0}}{2\epsilon} \left[1 + s\sqrt{1 - \frac{4\epsilon^2 v^2}{\sigma_{E0}^2} k^2}\right], \tag{8}$$

where $s = \pm 1$. The solutions for given $s$ are degenerate in $\lambda$, so we suppress the $\lambda$ subscript. The real (imaginary) parts of the solutions are depicted in Fig. S10 (a)[(b)] using the same parameters as for Fig. 4 of the Main Text: $\sigma_{E0} = 50\ \Omega^{-1}\ \mathrm{m}^{-1}$ and $\epsilon_r = 30$ (hence $v = c/\sqrt{30}$, where $c$ is the speed of light). There is a threshold wavenumber $k^* = \sigma_{E0}/2v\epsilon$ below which there is no propagation and the modes are purely decaying. Unsurprisingly, both modes are stable for all $k$, i.e. their amplitudes decay as $e^{\mathrm{Im}[\omega(k)]t}$ with $\mathrm{Im}[\omega(k)] < 0$.

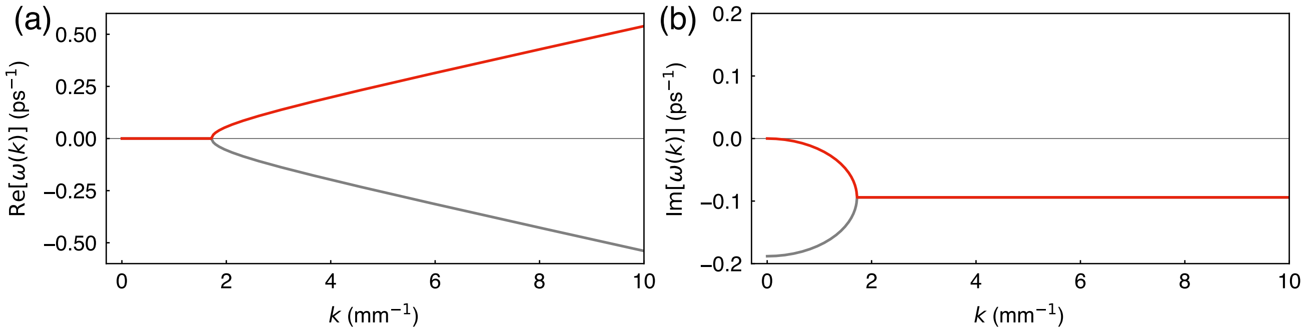


Fig. S10. **Ohmic conduction.** Real (a) and imaginary (b) parts of Eq. (8), where the red curve corresponds to $s = 1$ and the gray to $s = -1$. The red curve evolves into the non-propagating instability of Fig. S11 with the inclusion of the chiral magnetic effect.

**DC chiral magnetic effect.** Next, we add a DC chiral magnetic effect to the previous case, i.e. we put $\sigma_{\mathrm{E}}(\omega) = \sigma_{E0}$ and $\sigma_{\mathrm{M}}(\omega) = e^2\mu_{\mathrm{DC}}/4\pi^2\hbar^2$ [see Eq. (2) of the Main Text]. The dispersion relations become

$$\omega_{\lambda s}(k) = -\frac{i\sigma_{E0}}{2\epsilon}\left[1 + s\sqrt{1 - \frac{4\epsilon^2 v^2}{\sigma_{E0}^2}k\left(k - \lambda\frac{e^2\mu_{\mathrm{DC}}}{4\pi^2\hbar^2\epsilon v^2}\right)}\right], \tag{9}$$

as shown in Fig. S11 (a) for the real part and (b) for the imaginary part, using the same parameters as in Fig. 4 of the Main Text ($\sigma_{E0} = 50\ \Omega^{-1}\ \mathrm{m}^{-1}$, $\mu_{\mathrm{DC}} = 0.5\mathrm{eV}$, and $\epsilon_r = 30$). The $s = -1$, $\lambda = \mathrm{sign}(\mu_{\mathrm{DC}})$ branch is unstable ($\mathrm{Im}[\omega(k)] > 0$) for $0 < k < e^2|\mu_{\mathrm{DC}}|/4\pi^2\hbar^2\epsilon v^2$. In the limit $\sigma_{E0} \to 0$, this reproduces the result from Ref. [23] (see also [24]). However, this instability does not propagate, since $\mathrm{Re}[\omega(k)] = 0$ throughout the interval of $k$ for which the branch is unstable. It is therefore expected not to contribute to the radiation field outside the sample. As a consistency check, we note that Eq. (7b) with purely imaginary $\omega(k)$ implies that the Poynting vector $\boldsymbol{S} = \frac{1}{\mu_0}\mathrm{Re}[\boldsymbol{E}] \times \mathrm{Re}[\boldsymbol{B}]$ vanishes.

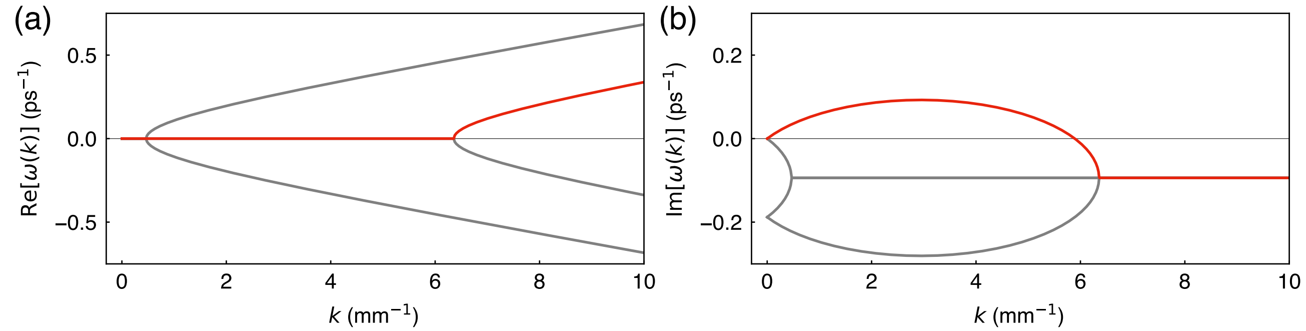


Fig. S11. **DC chiral magnetic effect with Ohm conductivity.** Real (a) and imaginary (b) parts of Eq. (9), where the red curve corresponds to $s = -1$ and $\lambda = \mathrm{sign}(\mu_{\mathrm{DC}})$ and features a non-propagating instability for sufficiently small wavenumbers.

**Hall effect.** Only time-reversal breaking Weyl semimetals/semiconductors can have an anomalous Hall effect in equilibrium. In time-reversal invariant tellurium, photoexcitation may give rise to a valley Hall effect [25], however, we expect it to be negligible in comparison to the classical Hall effect under an external magnetic field $B_0 > 1$ T. The classical Hall effect may be included in the preceding analysis by adding a term $\sigma_H \boldsymbol{E} \times \boldsymbol{B}_0$ to Eq. (4). We note that the observed THz emission is collected along a direction perpendicular to $\boldsymbol{B}_0$ within a cone of solid angle $\approx 0.6\pi$. However, for simplicity, we choose $\boldsymbol{k} = k\boldsymbol{B}_0/B_0$ and behavior is qualitatively similar for those $\boldsymbol{k}$ within the emission cone that have finite projection along $\boldsymbol{B}_0$. (However, when $\boldsymbol{k} \perp \boldsymbol{B}_0$, the instability does not propagate.) Repeating previous steps, one finds that the dispersion relations are determined by

$$\epsilon(\omega^2 - v^2k^2) + i\omega\sigma_{E0} + \lambda\left(\frac{e^2\mu_{\mathrm{DC}}}{4\pi^2\hbar^2}k - \omega\sigma_H B_0\right) = 0. \tag{10}$$

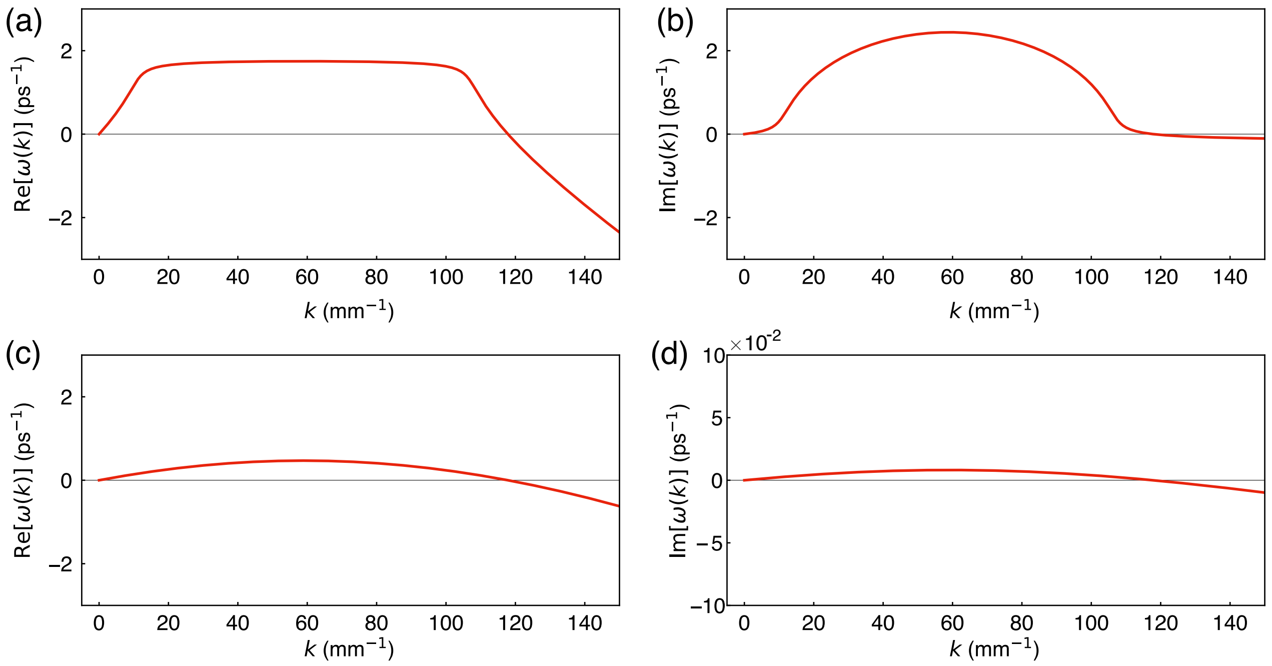


Fig. S12. **Hall effect with DC chiral magnetic effect and Ohm conductivity.** Real (a) and imaginary (b) parts of Eq. (11) with $B_0 = 1$ T, where the red curve corresponds to $s = -1$ and $\lambda = \mathrm{sign}(\mu_{\mathrm{DC}})$ and features a propagating instability for sufficiently small wavenumbers. For clarity, other dispersion relations are not shown. Plots (c) and (d) are the same but with $B_0 = 6$ T. Note the rescaled vertical axis in plot (d) compared to plots (a-c).

The solutions are [26]

$$\omega_{\lambda s}\ (k) = -i\frac{\sigma_{E0} + i\lambda\sigma_H B_0}{2\epsilon}\left[1 + s\sqrt{1 - \frac{4\epsilon^2 v^2}{(\sigma_{E0} + i\lambda\sigma_H B_0)^2}k\left(k - \lambda\frac{e^2\mu_{\mathrm{DC}}}{4\pi^2\hbar^2\epsilon v^2}\right)}\right]$$
$$\xrightarrow[s=-1]{} \frac{e^2\mu_{\mathrm{DC}}}{4\pi^2\hbar^2}\frac{1}{\sigma_{\mathrm{E}}^2 + \sigma_H^2 B_0^2}\ (\sigma_H B_0 + i\lambda\sigma_{\mathrm{E}})k + \mathcal{O}(k^2). \tag{11}$$

The $\mathcal{O}(k)$ truncation shows an unstable propagating mode when $\lambda = \mathrm{sign}(\mu_{\mathrm{DC}})$. However, without coupling to IR-active oscillators, this model implies that $\mathrm{Re}[\omega(k)]$ is not pinned and depends on $B_0$, contrary to the lack of $B_0$ dependence in the mode frequencies observed from the emissions. For example, taking $\sigma_{E0} = 100\ \Omega^{-1}\ \mathrm{m}^{-1}$, $\sigma_H = 10^3\ \Omega^{-1}\ \mathrm{m}^{-1}\ \mathrm{T}^{-1}$, $\mu_{\mathrm{DC}} = 10$ eV, $\epsilon = 30\epsilon_0$, the resulting dispersion relations for $B_0 = 1$ T and $B_0 = 6$ T are shown in Fig. S12 (a-b) and (c-d). Clearly, $\mathrm{Re}[\omega(k)]$ of the solution changes significantly from $B_0 = 1$ T [see Fig. S12 (a)] to $B_0 = 6$ T [see Fig. S12 (c)]. Additionally, for the oscillation frequency of this unstable mode to align with the mode frequency in THz emissions (approximately 1 $\mathrm{ps}^{-1}$) over the range of applied $B_0$, an unrealistically large value of $\mu_{\mathrm{DC}}$ ($>10^2$ eV) would be required. Furthermore, the predicted amplification rate is roughly of the same order as the oscillation frequency, as seen by comparing the imaginary part in Fig. S12 (b) with the real part in Fig. S12(a) for $B_0 = 1$ T, or Fig. S12 (d) with (c) for $B_0 = 6$ T. These observations are contrary to the experimental data, which shows that the amplification rate is around two orders of magnitude smaller than the oscillation frequency. We ignore the Hall effect and pursue a different possibility for the above reasons.

**Coupling to an IR-active oscillator.** Since the oscillator frequency of the amplifying component extracted from the THz emission data roughly agrees with that expected of a tellurium impurity level, we explore the possibility that an impurity dipole oscillator acquires instability via a coupling to the electron fluid. The mathematical descriptions are provided in the Main Text Eqs. (2) and (3). Specifically, we comment here that the form of Main Text Eq. (2) has been proposed in chiral metals [27], as well as Weyl semimetals given that $k \ll |\omega|/v_F$ ($v_F$ is the Fermi velocity) [26]. The upper bound of the valid $k$ region, as seen in Main Text Fig. 4, is safely much smaller than $|\omega|/v_F$, since $|\omega|/v_F \gtrsim 10^3\ \mathrm{mm}^{-1}$ given that $\omega \approx 2.5\ \mathrm{ps}^{-1}$ and $v_F \lesssim 10^6\ \mathrm{ms}^{-1}$.

The dispersion relations are the solutions of a quintic polynomial and cannot be written down analytically. Therefore, we present only numerical plots. In Fig. S13, we numerically calculate the model of the Main Text

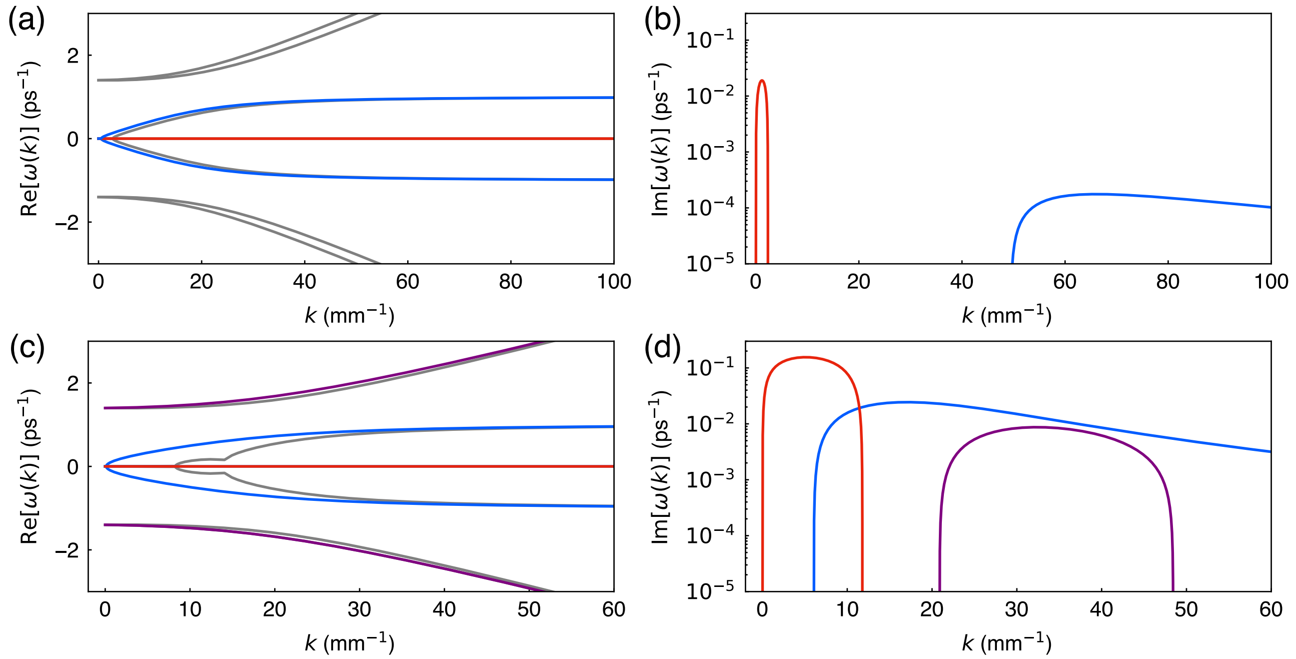


Fig. S13. **Coupling to an IR-active oscillator.** Real (a) and imaginary (b) parts of the dispersion relations for the model described in the Main Text, with $\mu_{\rm DC} = \mu_{\rm AC} = 0.2$ eV, demonstrating that the relative sign of $\mu_{\rm AC}$ and $\mu_{\rm DC}$ has little qualitative effect on the dispersion relations. Red: non-propagating instability. Blue: propagating instability. Plots (c) and (d) have $\mu_{\rm DC} = 1$eV and $\mu_{\rm AC} = -1$ eV. An additional branch of the dispersion relations (purple) becomes unstable.

with values of $\mu_{\rm DC}$ and $\mu_{\rm AC}$ that differ from Main Text Fig. 4 while keeping all other parameters identical ($\sigma_{E0} = 50\ \Omega^{-1}\ {\rm m}^{-1}$, $n = 10^{16}\ {\rm cm}^{-3}$, $\tau = 1$ ps, and $\epsilon = 30\epsilon_0$). Fig. S13(a-b) assumes $\mu_{\rm DC} = \mu_{\rm AC} = 0.2$ eV, whereas Fig. S13(c-d) assumes $\mu_{\rm DC} = 1$ eV, $\mu_{\rm AC} = -1$ eV.

Here we discuss the degeneracy and polarization of the plane-wave solutions. Maxwell's equations, with current $\boldsymbol{j}(\boldsymbol{r},t)$ linear in $\boldsymbol{E}(\boldsymbol{r},t)$ and $\boldsymbol{B}(\boldsymbol{r},t)$, are linear with real coefficients. Therefore, the complex conjugate of any solution $\{\boldsymbol{E}(\boldsymbol{r},t), \boldsymbol{B}(\boldsymbol{r},t)\}$ is also a solution. Applying this to the set of all plane-wave solutions $\boldsymbol{E}_{\lambda s\boldsymbol{k}}, \boldsymbol{B}_{\lambda s\boldsymbol{k}} \sim e^{i(\boldsymbol{k}\cdot\boldsymbol{r}-\omega_{\lambda s}(k)t)}$, we see that for each branch $s$ there must be a branch $s'$ such that $\omega_{\lambda s'}(k) = -\omega^*_{\lambda s}(k)$. For non-oscillatory modes ($\text{Re}[\omega_{\lambda s}(k)] = 0$), $s'$ can coincide with $s$, as in the case of the non-propagating instability of Eq.(9). On the other hand, each propagating mode $\lambda s$ ($\text{Re}[\omega_{\lambda s}(k)] \neq 0$) is accompanied by a distinct partner $\lambda s'$ whose dispersion relation has the same imaginary part but opposite real part, as can be seen in the gray, blue, and purple curves of Fig. S13 (a) and (c). Note that Fig. 4(a) of the Main Text shows only the branches with $\text{Re}[\omega_{\lambda s}(k)] > 0$ for clarity.

To better understand the structure of the modes, we can use isotropy to put $\boldsymbol{k} = k\hat{\boldsymbol{z}}$ with $k > 0$, $\boldsymbol{e}_1 = \hat{\boldsymbol{x}}$, and $\boldsymbol{e}_2 = \hat{\boldsymbol{y}}$ in Eq. (7) without loss of generality. Let the partner of a given mode $\lambda s$ be denoted as $\lambda s'$ (possibly with $s' = s$), so that $\omega_{\lambda s'}(k) = -\omega^*_{\lambda s}(k)$. Focusing for simplicity on the behavior of the magnetic field, we take the real part of Eq. (7) to find

$$\text{Re}[\boldsymbol{B}_{\lambda sk}(z,t)] = \lambda k\left[\cos\left(kz - \text{Re}[\omega_{\lambda s}(k)]t\right)\hat{\boldsymbol{x}} - \lambda\sin\left(kz - \text{Re}[\omega_{\lambda s}(k)]t\right)\hat{\boldsymbol{y}}\right]e^{\text{Im}[\omega_{\lambda s}(k)]t}. \tag{12}$$

Its partner is

$$\text{Re}[\boldsymbol{B}_{\lambda s'k}(z,t)] = \lambda k\left[\cos\left(kz + \text{Re}[\omega_{\lambda s}(k)]t\right)\hat{\boldsymbol{x}} - \lambda\sin\left(kz + \text{Re}[\omega_{\lambda s}(k)]t\right)\hat{\boldsymbol{y}}\right]e^{\text{Im}[\omega_{\lambda s}(k)]t}. \tag{13}$$

Similar expressions can be obtained for the electric fields. The solutions Eq. (12) and Eq. (13) are circularly polarized waves with the same helicity $\lambda$ but opposite propagation directions. Returning to arbitrary $\boldsymbol{k}$, we conclude that the solutions $\lambda s$ and $\lambda s'$, taken together, describe a single wave with definite helicity $\lambda$ that can propagate in any direction. The wave is decaying or amplifying according to the sign of $\text{Im}[\omega_{\lambda s(k)}]$.

Next, we discuss how changing the values of $\mu_{\rm AC}$ and $\mu_{\rm DC}$ affects the unstable solutions. When $\sigma_{\rm M}$ is zero, the solutions are doubly degenerate transverse waves. When $\sigma_{\rm M}$ is nonzero, the solutions of radiative instabilities

(due to $\mu_{\rm AC} \neq 0$) under the assumption of constant $\mu_{\rm DC}$ and $\mu_{\rm AC}$ require an energy source, which we attribute to a nonzero $\mu_{\rm DC}$. Therefore when we investigate cases where $\sigma_{\rm M} \neq 0$, we set $\mu_{\rm DC} \neq 0$ and $\mu_{\rm AC} \neq 0$ simultaneously. In Fig. S13 and Fig. 4 of the Main Text, the pair of propagating solutions shown in blue have $\lambda = \mathrm{sign}(\mu_{\rm AC})$, while the non-propagating solution shown in red has $\lambda = \mathrm{sign}(\mu_{\rm DC})$. The propagating solution with helicity $\lambda = -\,\mathrm{sign}(\mu_{\rm AC})$ remains stable. Flipping the sign of $\mu_{\rm AC}$ has minimal impact on the dispersion relations, primarily altering the helicity of the propagating instabilities. In particular, if $\mu_{\rm AC}$ is replaced by $+0.5$ eV in Fig. 4 of the Main Text, the conclusions drawn there remain largely unchanged. Notably, the increase of the absolute values of $\mu_{\rm AC}$ and $\mu_{\rm DC}$ can lead to additional propagating instability. As the parameters are tuned from that of Fig. S13 (a) and (b) to that of Fig. S13 (c) and (d), one of the higher-frequency stable solutions (gray) turns into the additional propagating instability (purple).

Finally, we comment on the observation of linearly polarized propagating instability in the THz range. A linearly polarized wave can be expressed as a superposition of left- and right-circularly polarized waves with equal amplitude; in this case, a polaritonic instability of definite helicity $\lambda = \mathrm{sign}(\mu_{\rm AC})$ and a decaying wave of opposite helicity $\lambda = -\,\mathrm{sign}(\mu_{\rm AC})$, both exhibiting similar phase velocities. The linear sum of the two circularly polarized components can mimic a linearly polarized instability provided that the amplification rate of the polaritonic instability and the damping rate of its decaying counterpart are both significantly smaller than the inverse of the observation time window.

**The effect of $\boldsymbol{B}_0$ and the initial excitation**. The $S_{\rm odd}$ amplitude is proportional to $|\boldsymbol{B}_0|$, which means that it is $\boldsymbol{B}_0$ that allows us to observe the emission in the first place, though the amplification behavior itself does not require the external field $\boldsymbol{B}_0$ - the static $\boldsymbol{B}_0$ does not lead to a dynamical component of $\boldsymbol{j}$ via a linear contribution $\sigma_{\rm M}\boldsymbol{B}_0$ (the above-discussed Hall effect is bilinear in fields). The initial excitation can be phenomenologically captured by the magnetoelectric coupling $\boldsymbol{P} = \frac{1}{\mu_0}\Delta \overset{\leftrightarrow}{\alpha}\, \boldsymbol{B}_0$, which describes the linear response of bounded dipoles to the external fields, producing the observed $S_{\rm odd}$ coherent oscillations at multiple frequencies [28]. The tensor $\Delta \overset{\leftrightarrow}{\alpha}$ corresponds to a sudden change in the magnetoelectric coupling coefficient around $t = 0$, which is due to photoexcited carrier dynamics that changes the spin-orbit coupling and the Rashba effect in tellurium. Note that the magnetoelectric coupling term, $\overset{\leftrightarrow}{\alpha}\, \boldsymbol{B}$, describes a bounded dipole, whereas the magneto-chiral current term $\sigma_{\rm M}\boldsymbol{B}$ describes a free current, and thus $\sigma_{\rm M}$ is not considered in the excitation of the bounded dipole. The magnitude of $\Delta \overset{\leftrightarrow}{\alpha}$ ($\alpha_{zz}$ when $z$ denotes the $\boldsymbol{B}_0$ direction), can be estimated from the experiment. From the magnitude of electro-optic sampling signal under a field of 6 T [29], we estimate the $\boldsymbol{B}_0$-antisymmetrized THz electric field at the sample to be $\boldsymbol{E}_{\rm rad} = 0.1$ V/cm, which corresponds to an estimated current density $|\boldsymbol{j}|$ of $6{\times}10^5$A/m$^2$ [30] and $\alpha_{zz} \approx 1$ ps$\cdot$m$^{-1}$, which is reasonable considering the magnitude of terahertz-range magnetoelectric coupling coefficients in materials [31]. Since $\frac{\omega\alpha_{zz}}{\mu_0} \ll \sigma_{\rm M}$, $\overset{\leftrightarrow}{\alpha}$ is not considered along with the magneto-chiral effect in the calculation.

[1] H. Barkhuijsen, R. de Beer, W. Bovée, and D. van Ormondt, Retrieval of frequencies, amplitudes, damping factors, and phases from time-domain signals using a linear least-squares procedure, Journal of Magnetic Resonance (1969) **61**, 465 (1985).

[2] B. P. Epps and E. M. Krivitzky, Singular value decomposition of noisy data: noise filtering, Experiments in Fluids **60**, 1 (2019).

[3] B. P. Epps and E. M. Krivitzky, Singular value decomposition of noisy data: mode corruption, Experiments in Fluids **60**, 1 (2019).

[4] J. J. Led and H. Gesmar, Application of the linear prediction method to nmr spectroscopy, Chemical reviews **91**, 1413 (1991).

[5] Y. Huang, S. Yang, S. Teitelbaum, G. De la Peña, T. Sato, M. Chollet, D. Zhu, J. L. Niedziela, D. Bansal, A. F. May, A. M. Lindenberg, O. Delaire, D. A. Reis, and M. Trigo, Observation of a novel lattice instability in ultrafast photoexcited snse, Phys. Rev. X **12**, 011029 (2022).

[6] Y. Huang, J. D. Querales-Flores, S. W. Teitelbaum, J. Cao, T. Henighan, H. Liu, M. Jiang, G. De la Peña, V. Krapivin, J. Haber, T. Sato, M. Chollet, D. Zhu, T. Katayama, R. Power, M. Allen, C. R. Rotundu, T. P. Bailey, C. Uher, M. Trigo, P. S. Kirchmann, E. D. Murray, Z.-X. Shen, I. Savić, S. Fahy, J. A. Sobota, and D. A. Reis, Ultrafast measurements of mode-specific deformation potentials of $Bi_2Te_3$ and $Bi_2Se_3$, Phys. Rev. X **13**, 041050 (2023).

[7] Y. Huang, S. Teitelbaum, S. Yang, G. De la Peña, T. Sato, M. Chollet, D. Zhu, J. L. Niedziela, D. Bansal, A. F. May, A. M. Lindenberg, O. Delaire, M. Trigo, and D. A. Reis, Nonthermal bonding origin of a novel photoexcited lattice instability in SnSe, Phys. Rev. Lett. **131**, 156902 (2023).

[8] R. Kumaresan and D. Tufts, Estimating the parameters of exponentially damped sinusoids and pole-zero modeling in noise, IEEE transactions on acoustics, speech, and signal processing **30**, 833 (1982).

[9] S. W. Teitelbaum, T. Henighan, Y. Huang, H. Liu, M. P. Jiang, D. Zhu, M. Chollet, T. Sato, E. D. Murray, S. Fahy, S. O'Mahony, T. P. Bailey, C. Uher, M. Trigo, and D. A. Reis, Direct measurement of anharmonic decay channels of a coherent phonon, Phys. Rev. Lett. **121**, 125901 (2018).

[10] J. Chesnoy and A. Mokhtari, Resonant impulsive-stimulated raman scattering on malachite green, Phys. Rev. A **38**, 3566 (1988).

[11] T. Dekorsy, H. Auer, H. J. Bakker, H. G. Roskos, and H. Kurz, Thz electromagnetic emission by coherent infrared-active phonons, Phys. Rev. B **53**, 4005 (1996).

[12] N. Kamaraju, S. Kumar, M. Anija, and A. K. Sood, Large-amplitude chirped coherent phonons in tellurium mediated by ultrafast photoexcited carrier diffusion, Phys. Rev. B **82**, 195202 (2010).

[13] G. Jnawali, Y. Xiang, S. M. Linser, I. A. Shojaei, R. Wang, G. Qiu, C. Lian, B. M. Wong, W. Wu, P. D. Ye, *et al.*, Ultrafast photoinduced band splitting and carrier dynamics in chiral tellurium nanosheets, Nature Communications **11**, 3991 (2020).

[14] Y. Couder, M. Hulin, and H. Thomé, Cyclotron resonance in tellurium, Phys. Rev. B **7**, 4373 (1973).

[15] K. Natori, T. Ando, M. Tsukada, K. Nakao, and Y. Uemura, The acceptor states in tellurium, Journal of the Physical Society of Japan **34**, 1263 (1973).

[16] T. Tani and S. Tanaka, Pressure effect on the impurity state and impurity conduction in tellurium, in *The Physics of Selenium and Tellurium: Proceedings of the International Conference on the Physics of Selenium and Tellurium, Königstein, Fed. Rep. of Germany, May 28–31, 1979* (Springer, 1979) pp. 142–152.

[17] D. Thanh, Effective mass approximation for acceptors in tellurium, Solid State Communications **9**, 631 (1971).

[18] Creative Commons Attribution 4.0 International Public License (CC BY 4.0) (2013).

[19] K. von Klitzing and J. Tuchendler, Impurity states of tellurium in high magnetic fields, in *Physics in High Magnetic Fields: Proceedings of the Oji International Seminar Hakone, Japan, September 10–13, 1980* (Springer, 1981) pp. 139–148.

[20] M. Sakano, M. Hirayama, T. Takahashi, S. Akebi, M. Nakayama, K. Kuroda, K. Taguchi, T. Yoshikawa, K. Miyamoto, T. Okuda, K. Ono, H. Kumigashira, T. Ideue, Y. Iwasa, N. Mitsuishi, K. Ishizaka, S. Shin, T. Miyake, S. Murakami, T. Sasagawa, and T. Kondo, Radial spin texture in elemental tellurium with chiral crystal structure, Phys. Rev. Lett. **124**, 136404 (2020).

[21] A. Koma and S. Tanaka, Etch pits and crystal structure of tellurium, Physica Status Solidi (B) **40**, 239 (1970).

[22] Y. Tanaka, S. Collins, S. Lovesey, M. Matsumami, T. Moriwaki, and S. Shin, Determination of the absolute chirality of tellurium using resonant diffraction with circularly polarized x-rays, Journal of Physics: Condensed Matter **22**, 122201 (2010).

[23] Y. Akamatsu and N. Yamamoto, Chiral plasma instabilities, Phys. Rev. Lett. **111**, 052002 (2013).

[24] I. A. Shovkovy, Anomalous plasma: chiral magnetic effect and all that, in *Peter Suranyi 87th Birthday Festschrift A Life in Quantum Field Theory* (World Scientific, 2023) pp. 291–316.

[25] K. F. Mak, K. L. McGill, J. Park, and P. L. McEuen, The valley hall effect in $MoS_2$ transistors, Science **344**, 1489 (2014).

[26] T. Amitani and Y. Nishida, Dynamical chiral magnetic current and instability in weyl semimetals, Phys. Rev. B **107**, 014302 (2023).

[27] S. Zhong, J. E. Moore, and I. Souza, Gyrotropic magnetic effect and the magnetic moment on the fermi surface, Phys. Rev. Lett. **116**, 077201 (2016).

[28] The infrared radiation is not generated through a magnetophotogalvanic effect due to NIR pump optical field $\tilde{\boldsymbol{E}}$, $\boldsymbol{P}_i = G^{(\mathrm{lin})}_{ijkl}\ (\tilde{\boldsymbol{E}}_j\tilde{\boldsymbol{E}}^*_k + \tilde{\boldsymbol{E}}^*_j\tilde{\boldsymbol{E}}_k)\boldsymbol{B}_{0,l} + G^{(\mathrm{circ})}_{ikl}\ (\tilde{\boldsymbol{E}} \times \tilde{\boldsymbol{E}}^*)_k\boldsymbol{B}_{0,l}$: $\tilde{\boldsymbol{E}}_{\mathrm{LCP}}$ and $\tilde{\boldsymbol{E}}_{\mathrm{RCP}}$ pumps produce negligible differences in THz emissions, indicating $G^{(\mathrm{circ})}_{ikl} \approx 0$, the THz emissions under different combinations of pump polarizations and sample orientations do not respect the symmetry of $G^{(\mathrm{lin})}_{ijkl}$ [32].

[29] We use the following parameters for CdTe: the (110)-cut CdTe crystal has a thickness $L$ of 1 mm and is approximately transparent for the THz range emission, its refractive index at the optical range is $n = 2.8$ [33], the electro-optic coefficient $r_{41}$= 4.5 pm/V [34]. We also consider the collection loss due to a finite solid angle covered by the lens, as well as the propagation loss.

[30] We consider the following parameters for tellurium: the THz-range refractive index $n_{\mathrm{THz}}$=5, the optical penetration depth at 1.2 eV is 300 nm at normal incidence [35].

[31] F. Y. Gao, X. Peng, X. Cheng, E. Viñas Boström, D. S. Kim, R. K. Jain, D. Vishnu, K. Raju, R. Sankar, S.-F. Lee, M. A. Sentef, T. Kurumaji, X. Li, P. Tang, A. Rubio, and E. Baldini, Giant chiral magnetoelectric oscillations in a van der waals multiferroic, Nature **632**, 273 (2024).

[32] S. V. Gallego, J. Etxebarria, L. Elcoro, E. S. Tasci, and J. M. Perez-Mato, Automatic calculation of symmetry-adapted tensors in magnetic and non-magnetic materials: a new tool of the bilbao crystallographic server, Acta Crystallographica Section A: Foundations and Advances **75**, 438 (2019).

[33] P. Hlıdek, J. Bok, J. Franc, and R. Grill, Refractive index of CdTe: Spectral and temperature dependence, Journal of Applied Physics **90**, 1672 (2001).

[34] B. Pradarutti, G. Matthäus, S. Riehemann, G. Notni, S. Nolte, and A. Tünnermann, Highly efficient terahertz electro-optic sampling by material optimization at 1060 nm, Optics Communications **281**, 5031 (2008).

[35] S. Tutihasi, G. Roberts, R. Keezer, and R. Drews, Optical properties of tellurium in the fundamental absorption region, Physical Review **177**, 1143 (1969).
